# Supplementary material for: Grammar-based Neural Text-to-SQL Generation
Source: arXiv:1905.13326 source file (2019-05-30)
Supplement: Supplementary file 1 [file 8supplementary-material.tex]

\appendix 

\section{Supplemental Material}
\label{sec:supplemental}

\begin{table}[]
\begin{tabular}{@{}lccc@{}}
\textbf{Dataset}                               & \textbf{Original} & \textbf{Unique} & \textbf{\%}      \\ \midrule
\textbf{Scholar} \\
\textbf{Query Split}        &          &              &         \\ \midrule
Dev                                   & 94       & 90           & 4.26\%  \\
Test                                  & 315      & 295          & 6.35\%  \\
Train                                 & 408      & 383          & 6.13\%  \\
\textbf{Question Split}     &          &              &         \\ \midrule
Dev                                   & 100      & 99           & 1.00\%  \\
Test                                  & 218      & 214          & 1.83\%  \\
Train                                 & 499      & 485          & 2.81\%  \\
\textbf{Restaurants} \\
\textbf{Query Split}    &          &              &         \\ \midrule
0                                     & 27       & 9            & 66.67\% \\
1                                     & 15       & 5            & 66.67\% \\
2                                     & 51       & 17           & 66.67\% \\
3                                     & 48       & 15           & 68.75\% \\
4                                     & 6        & 2            & 66.67\% \\
5                                     & 15       & 5            & 66.67\% \\
6                                     & 15       & 5            & 66.67\% \\
7                                     & 81       & 27           & 66.67\% \\
8                                     & 45       & 15           & 66.67\% \\
9                                     & 75       & 25           & 66.67\% \\
\textbf{Question Split} &          &              &         \\ \midrule
0                                     & 38       & 36           & 5.26\%  \\
1                                     & 38       & 38           & 0.00\%  \\
2                                     & 38       & 35           & 7.89\%  \\
3                                     & 38       & 35           & 7.89\%  \\
4                                     & 38       & 34           & 10.53\% \\
5                                     & 38       & 37           & 2.63\%  \\
6                                     & 38       & 32           & 15.79\% \\
7                                     & 38       & 31           & 18.42\% \\
8                                     & 37       & 32           & 13.51\% \\
9                                     & 37       & 34           & 8.11\%  \\
\textbf{ATIS} \\
\textbf{Query Split}           &          &              &         \\ \midrule
Dev                                   & 121      & 115          & 4.96\%  \\
Test                                  & 347      & 327          & 5.76\%  \\
Train                                 & 4812     & 4450         & 7.52\%  \\
\textbf{Question Split}        &          &              &         \\ \midrule
Dev                                   & 486      & 483          & 0.62\%  \\
Test                                  & 447      & 411          & 8.05\%  \\
Train                                 & 4347     & 4054         & 6.74\%  \\ \bottomrule
\end{tabular}
\caption{Duplicated queries in the Scholar, Restaurants and context-dependent ATIS datasets provided in \citep{FineganDollak2018ImprovingTE}. Duplicate queries biases evaluation metrics, as subsets of queries may be of different difficulty.}
\end{table}

\subsection{A Note on Text-to-SQL Datasets}
During a period of initial investigation for this work, we looked into the suitability of several text-to-SQL datasets recently proposed by \citep{FineganDollak2018ImprovingTE}, specifically restaurants \citep{data-restaurants-original}, Yelp, IMDB \citep{data-sql-imdb-yelp}, Geography \citep{data-geography-original}, Scholar \citep{data-atis-geography-scholar}, Academic \citep{data-academic} and Advising \citep{FineganDollak2018ImprovingTE}. Unfortunately, for a variety of reasons, we found several of these datasets unsuitable for our analysis. 

The interesting analysis of \citep{FineganDollak2018ImprovingTE} demonstrate that evaluation on the question split of above datasets only evaluates lexical generalization, due to the presence of SQL query templates which are common across train, test and development splits, which they use as motivation for the high accuracy of semantic parsing models across the standard splits of many datasets. While we agree with this general analysis, we find that several datasets contain exactly the same queries across splits, simply demonstrating erroneous construction of the original datasets.

Due to the high quality annotation our grammar-based approach requires (gold SQL queries must be parsed via a grammar - they are not considered as a string of tokens), we discovered several problems with the existing datasets which are not discussed by \citep{FineganDollak2018ImprovingTE}. In particular, we find that:

\begin{itemize}
    \item The question split of the Restaurants dataset is completely unsuitable for the evaluation of semantic parsing models due to systemic train/test overlap.
    \item Many of the dataset splits contain exactly duplicate questions (and questions which only differ in capitalization, which will result in exact duplication in practice), which introduce bias in the evaluation of models.
    \item The Advising dataset contains relative lexical references to dates which change throughout the dataset (e.g "last year" referring to many, non-canonicalized years). The authors of this dataset \citep{FineganDollak2018ImprovingTE} are aware of this deficiency and will fix the dataset in due course.

\end{itemize}

In particular, it appears that performance on the original (question based) split of the Restaurants dataset has always been greater than or equal to 98 \%, leading us to think that this problem identified with train/test leakage has been present since the dataset's conception. 

\begin{table}
\centering
\begin{tabular}{@{}l{0.5cm}p{0.2cm}p{0.2cm}p{0.2cm}p{0.2cm}p{0.2cm}p{0.2cm}p{0.2cm}p{0.2cm}p{0.2cm}@{}}
\toprule
Split & 1  & 2  & 3  & 4  & 5  & 6  & 7  & 8  & 9  & 10 \\ \midrule
1             & 38 & 7  & 7  & 6  & 11 & 8  & 8  & 8  & 5  & 8  \\
2             & 7  & 38 & 4  & 16 & 10 & 8  & 4  & 9  & 6  & 9  \\
3             & 8  & 4  & 38 & 7  & 7  & 7  & 7  & 5  & 10 & 10 \\
4             & 6  & 16 & 7  & 38 & 6  & 9  & 4  & 7  & 5  & 7  \\
5             & 13 & 10 & 7  & 6  & 38 & 9  & 7  & 7  & 7  & 6  \\
6             & 8  & 8  & 6  & 8  & 8  & 38 & 8  & 6  & 9  & 10 \\
7             & 10 & 5  & 8  & 4  & 7  & 8  & 38 & 6  & 9  & 5  \\
8             & 7  & 11 & 5  & 7  & 6  & 7  & 7  & 38 & 6  & 5  \\
9             & 6  & 6  & 12 & 6  & 5  & 10 & 8  & 6  & 37 & 5  \\
10            & 8  & 9  & 11 & 7  & 7  & 10 & 5  & 4  & 5  & 37 \\ \bottomrule
\end{tabular}
\caption{Split overlap in the Restaurants dataset (question split only). Note that this matrix should be diagonal.}
\end{table}

\begin{figure}
  \centering
\begin{lstlisting}[basicstyle=\fontfamily{cmtt}\small,columns=fullflexible,frame=bt,  breaklines=true]
query = (ws "(" ws "SELECT" ws distinct ws select_results ws "FROM" ws table_refs ws where_clause ws group_by_clause ws ")" ws) / (ws "(" ws "SELECT" ws distinct ws select_results ws "FROM" ws table_refs ws where_clause ws ")" ws) / (ws "SELECT" ws distinct ws select_results ws "FROM" ws table_refs ws where_clause ws)
select_results = col_refs / agg
agg = (agg_func ws "(" ws col_ref ws ")") / (agg_func ws "(" ws col ws ")")
agg_func = "MIN" / "min" / "MAX" / "max" / "COUNT" / "count"
col_refs = (col_ref ws "," ws col_refs) / col_ref
table_refs = (table_name ws "," ws table_refs) / table_name
where_clause = ("WHERE" ws "(" ws conditions ws ")" ws) / ("WHERE" ws conditions ws)
group_by_clause = "GROUP" ws "BY" ws col_ref
conditions = (condition ws conj ws conditions) / (condition ws conj ws "(" ws conditions ws ")") / ("(" ws conditions ws ")" ws conj ws conditions) / ("(" ws conditions ws ")") / ("not" ws conditions ws) / ("NOT" ws conditions ws) / condition
condition = in_clause / ternaryexpr / biexpr
in_clause = ws col_ref ws "IN" ws query ws
biexpr = ( col_ref ws binaryop ws value) / (value ws binaryop ws value)
binaryop = "+" / "-" / "*" / "/" / "=" / ">=" / "<=" / ">" / "<" / "is" / "IS"
ternaryexpr = (col_ref ws "not" ws "BETWEEN" ws value ws "AND" ws value ws) / (col_ref ws "NOT" ws "BETWEEN" ws value ws "AND" ws value ws) / (col_ref ws "BETWEEN" ws value ws "AND" ws value ws)
value = ("not" ws pos_value) / ("NOT" ws pos_value) / pos_value
pos_value = ("ALL" ws query) / ("ANY" ws query) / number / boolean / col_ref / agg_results / "NULL"
agg_results = (ws "(" ws "SELECT" ws distinct ws agg ws "FROM" ws table_name ws where_clause ws ")" ws) / (ws "SELECT" ws distinct ws agg ws "FROM" ws table_name ws where_clause ws)
boolean = "true" / "false"
ws = ~"\s*"iu
conj = "AND" / "OR"
distinct = "DISTINCT" / ""
\end{lstlisting}
  \vspace{-2mm}
  \caption{The base SQL grammar before augmentation with schema specific and utterance specific rules \jonathan{will you make a prettier version?}}
  \label{fig:atis_grammar_full}
  \vspace{-5mm}
\end{figure}

\begin{figure}[t]
  \centering
\begin{lstlisting}[basicstyle=\fontfamily{cmtt}\small,columns=fullflexible,frame=bt,  breaklines=true]
city_city_name_string = "'WESTCHESTER COUNTY'" / "'DETROIT'" 

city_city_code_string =  "'HHPN'" / "'DDTT'" 

table_name = "state" / "restriction" / "month" / "ground_service" / "food_service" / "flight_stop" / "flight_leg" / "flight_fare" / "flight" / "fare_basis" / "fare" / "equipment_sequence" / "days" / "date_day" / "class_of_service" / "city" / "airport_service" / "airport" / "airline" / "aircraft"

biexpr = ("state" ws "." ws "state_name" ws binaryop ws state_state_name_string) / ("state" ws "." ws "state_code" ws binaryop ws state_state_code_string) / ("restriction" ws "." ws "restriction_code" ws binaryop ws restriction_restriction_code_string) / ("ground_service" ws "." ws "transport_type" ws binaryop ws ground_service_transport_type_string) / ("food_service" ws "." ws "meal_description" ws binaryop ws food_service_meal_description_string) / ("food_service" ws "." ws "compartment" ws binaryop ws food_service_compartment_string) / ("flight_stop" ws "." ws "stop_airport" ws binaryop ws flight_stop_stop_airport_string) / ("flight" ws "." ws "flight_days" ws binaryop ws flight_flight_days_string) / ("flight" ws "." ws "airline_code" ws binaryop ws flight_airline_code_string) / ("fare_basis" ws "." ws "fare_basis_code" ws binaryop ws fare_basis_fare_basis_code_string) / ("fare_basis" ws "." ws "economy" ws binaryop ws fare_basis_economy_string) / ("fare_basis" ws "." ws "class_type" ws binaryop ws fare_basis_class_type_string) 

\end{lstlisting}
  \vspace{-2mm}
  \caption{Example of additional rules added to the base SQL grammar based on database schema and entities in utterance if the entities \texttt{WESTCHESTER COUNTY} and \texttt{DETROIT} are detected in the utterance}
  \label{fig:additional_grammar_rules_full}
  \vspace{-5mm}
\end{figure}
